# Supplementary material for: Breaking the k/log k Barrier in Collective Tree Exploration via Tree-Mining
Source: arXiv:2309.07011 source file (2023-10-30)
Supplement: Supplementary file 1 [file appendix.tex]

\section{Ignore Appendix!!}
\section{Tree-mining Lower Bounds}
We need a novel exploration model, where the number of available edges is not known upon arrival. The goal of this section is to motivate the locally greedy setting.

\paragraph{Exploration model.} When located at a node $v$, robots have query the node for a new dangling edge. If none is available, the node is considered finished. While one is available, the robot does not know how many \textit{more} dangling edges there might be at this node. For this model, where the information is restricted, our algorithm seem to be optimal.

Another possible exploration model is one with waiting times at all nodes that are completely unknown. And this time is divided by the number of robots present at this node. i.e. there is some work to be done at all nodes (mining).

\subsection{Lower bound}
\begin{theorem}\label{th: reduction-reverse} 
A strategy $s_2$ of the adversary implies that for any depth $D$ and number of robots $k$, for any locally greedy exploration algorithm, there exists a tree $T$ of depth $D$ that which exploration takes at least, 
$$\frac{2n}{k}+\frac{g_k(s_2, D)}{k}+D,$$
where we do not control the number of nodes $n$.
\end{theorem}
\begin{proof}[Proof of Theorem \ref{th: reduction-reverse}] Sketch of proof.

\begin{itemize}
    \item We consider a locally greedy exploration algorithm $\Acal$. We will build a tree with diameter $D$ that satisfies the property described above. 
    \item When a node is killed, we consider the ``freed" robots, those which have a behaviour that is not entirely specified by the algorithm. 
    \item While these robots are located on a killed node, we block the other robots at their current position by providing them with sufficiently many neighbours to explore.
    \item Once they all reach a non-killed node, we refer to this non-killed node as their target. We use this assignment as the strategy of player 1.
    \item We use the strategy of player 2 to decide which robots are allowed to terminate. 
    \item \rc{we need some additional assumption, that the robots are blind to the number of adjacent edges. It is for this kind of algorithm that our lower bounds hold. }
\end{itemize}    
\end{proof}

\subsection{Tree-mining lower-bounds}
\begin{theorem} \label{th: lbk}
    There exists a strategy $s_2$ for the adversary such that $\forall k, D: \ell_k(s_2,D) \geq Dk\ln(k).$
\end{theorem}

\proof[Proof of Theorem \ref{th: lbk}]{
We now turn to proving a lower-bound on the tree-mining game. 
\begin{itemize}
    \item Start by splitting $k$ pebbles into $k$ subgroups.
    \item Then always kill the subgroup with the biggest amount of pebble, until there is one group left.
    \item This will lead to a cost of $k\ln(k)$, when the player uses the strategy. 
    \item Do this at all depth. 
    \item This leads to a $k\ln(k)D$ cost.
\end{itemize}

}
\begin{proposition}
    Consider a locally greedy exploration algorithm, that achieves additive error $f(k,D)$ factorizing as 
    $$f(k,D) = h(k)g(D),$$
    then $h(k)\geq \ln(k)$ and $g(D)\geq D$.
\end{proposition}
Though trivial given the statement above, this result implies that there does not exists a $2n/k+D^2$ (locally greedy) exploration algorithm, thereby partially answering an open question of \cite{cosson2023breadth}. This suggests that the $\texttt{BFDN}$ strategy of complexity $2n/k+D^2\ln(k)$ achieves some form of optimality (in $k$). This also seems to highlight that the settings of collaborative exploration where an upper-bound is given for $n$, such as $n\leq k$ in \cite{disser2017general} or $Dn^c\leq k$ in \cite{dereniowski2015fast} are intrinsinquely different. Indeed, there is as simple $D^2$ algorithm for the latter, and a $O(D)$ algorithm for the former.

\paragraph{Comparison with known lower bounds.}
For a given strategy $s_2\in \Scal_2$, we define $g_k(s_2,D)$ as follows,
\begin{align*}
g_k(s_2,D) &= \min_{s_1 \in \Scal_1} \score(s_1,s_2,D).
\end{align*} 

\section{Additional ideas to investigate}
\subsection{Optimizing the competitive ratio, given some additive overhead}
This does not seem to give any result. 
\subsection{Discussion on the generality of locally-greedy exploration algorithms}
In this paragraph, we discuss on the generality of the class of locally-greedy exploration algorithm among exploration algorithm. We first note that the term ``locally-greedy'' may well qualify any offline exploration algorithm. This yields the following observation.

\begin{proposition}
    For any tree $T$, with $n$ nodes and depth $D$ there exists a locally greedy exploration algorithm that explores the tree in time $\frac{2n}{k}+2D$. \rc{FALSE as is}
\end{proposition}
\begin{proof}
The proof is largely inspired from the offline exploration strategy proposed in \cite{dynia2006power}. Consider a depth-first path of the tree $T$. This path goes through $n$ edges. 
\rc{This result is also questionable actually}
We seem to have a problem. It would be interesting to devise another offline strategy that would be locally greedy. For instance, it could work in such a way that for any node, the number of children is known and the robots try to balance the number of robots per children!! This is a setting that is somewhere between the offline and the online setting and its study would be of interest. 
\end{proof}

Then, thanks to Yao's minimax principle, any randomized algo on locally greedy algorithm suffice. Meaning that it will be close to acheiving the best that a randomized algo on non-locally greedy algorithms.

\subsection{Implementation with limited communication}
Teams of robots are independants, and they can share information at the lowest common ancestor, at no additional cost. Thus can be implemented with local comm. (there is an induction to make)
\subsection{Randomized strategies for the tree-mining problem}
Does randomization help at all? We could imagine there is a waiting time on all nodes at which it will break into pieces (the number of pieces and the time are fixed a priori) can we do any better?

A way to frame the problem in the competitive analysis framework is as follows. Goal is for $k$ miners to reach depth $D$ while minimizing the number of overlapping movements (if two miners move in the same edge, only one of both will get the revenue from it). With hindsight, an offline algorithm achieves this in $(k-1)D$. Without hindsight, how does an online algorithm competes? 

\section{old stuff}
One advantage of locally greedy algorithms is that robots do not use the information of the precise number of dangling edges 

Another advantage of locally greedy algorithms is that they do not use the knowledge

Locally greedy are particularly suited for a more complex setting where agents do not have the ability to see the number of a children that some node has when they arrive. But simply see if the node is saturated or not. - %If we add the assumption that free robots must move in the direction of some dangling edge, we have the property that the algo terminates \rc{actually, we would need to add that the robot cannot backtrack, or alternatively that it is anchored at some point} In this paper, we posit that the study of collaborative exploration can be restricted to the study of locally greedy algorithms.

%\rc{We will motivate locally greedy algo by saying that they solve the limited feedback problem}

%\begin{definition}
%    A reasonable algorithm is an exploration algorithm such that all robots move in a direction leading to some dangling edge. 
%\end{definition}
%\rc{Maybe a better name would be ``restless'' algorithm, for they always move to a dangling edge and do not backtrack}
%\rc{another option is to say that if there is a single robot that is free of its movements, it is not allowed to backtrack}

\subsection{Implications on the competitive ratio.}
In this section, we explain how the results above entail a $\mathcal{O}\left(k/\exp\left(\sqrt{\ln(k)}\right)\right)$ competitive algorithm for collaborative tree exploration. Note that quite surprisingly, this exploration algorithm uses a fraction $h(k)<k$ of the robots, while all remaining $k-k'$ robots remain posted at the root.  
\begin{lemma}
    If there exists a $\frac{2n}{k}+\mathcal{O}\left(\exp(\alpha \ln(k)^2)D\right)$ $k$-exploration algorithm, then using this algorithm with only $h(k) = \ceil{\exp\left(\delta\sqrt{\ln{k}}\right)}$ searchers, with $\alpha\delta^2<1$, and keeping the remaining $k-h(k)$ searchers inactive at the root yields a competitive ratio of $\mathcal{O}\left(\frac{k}{h(k)}\right)$. 
\end{lemma}
\begin{proof}
    The runtime of the associated algorithm is bounded by,
    \begin{equation*}
        \frac{2n}{h(k)}+C\exp(\alpha \ln(h(k))^2)D,
    \end{equation*}
    for some constant $C$. We note that $\exp(\alpha\ln(h(k))^2)$ is asymptotically equivalent to $\exp(\alpha\delta^2\ln(k)) = k^{\alpha\delta^2}$. Since $\alpha\delta^2<1$, the runtime is bounded by,
    \begin{equation*}
        \frac{2n}{h(k)}+\mathcal{O}\left(k^{\alpha\delta^2}D\right) = \mathcal{O}\left(\frac{k}{h(k)}\right)\left(\frac{n}{k}+D\right).
    \end{equation*}
\end{proof}

A direct consequence of this result applied to $\alpha = 1/\ln(2)$ is the following,
\begin{theorem}
    There exists a $\mathcal{O}\left(\frac{k}{\exp\left(0.8\sqrt{\ln(k)}\right)}\right)$-competitive algorithm for the collaborative tree exploration problem.
\end{theorem}
